# Supplementary material for: Hybrid Quantum-Classical Photonic Neural Networks
Source: arXiv:2407.02366 source file (2024-07-14)
Supplement: Supplementary file 1 [file supplementary_information.tex]

\begin{filecontents}{supplementary_information.aux}
\relax 
\citation{weedbrook_gaussian_2012}
\citation{killoran_strawberry_2019}
\citation{kok_introduction_2010}
\citation{killoran_strawberry_2019}
\citation{gerry_introductory_2005}
\citation{killoran_strawberry_2019}
\citation{hayman_hybrid_2022}
\citation{hayman_hybrid_2022}
\@writefile{toc}{\contentsline {section}{\numberline {I}Simulation and Cutoff Dimension}{1}{}}
\newlabel{sec:simulation_cutoff}{{I}{1}{}{}{}}
\citation{hayman_hybrid_2022}
\citation{hayman_hybrid_2022}
\@writefile{toc}{\contentsline {section}{\numberline {II}CV Gates}{2}{}}
\newlabel{sec:gates}{{II}{2}{}{}{}}
\@writefile{lot}{\contentsline {table}{\numberline {I}{\ignorespaces Table describing the different gate operations in a CV quantum circuit \cite  {hayman_hybrid_2022}. For reference $\mathcal  {U}$ is made up of beamsplitter and rotation gates to form an N-port interferometer. In the text the symbol for the kerr gate was $\Phi $ while here it is $K$.\relax }}{2}{}}
\providecommand*\caption@xref[2]{\@setref\relax\@undefined{#1}}
\newlabel{tab:gates}{{I}{2}{}{}{}}
\newlabel{fig:vacuum}{{1a}{2}{}{}{}}
\newlabel{sub@fig:vacuum}{{a}{2}{}{}{}}
\newlabel{fig:displacement}{{1b}{2}{}{}{}}
\newlabel{sub@fig:displacement}{{b}{2}{}{}{}}
\newlabel{fig:squeezing}{{1c}{2}{}{}{}}
\newlabel{sub@fig:squeezing}{{c}{2}{}{}{}}
\newlabel{fig:rotation}{{1d}{2}{}{}{}}
\newlabel{sub@fig:rotation}{{d}{2}{}{}{}}
\newlabel{fig:kerr}{{1e}{2}{}{}{}}
\newlabel{sub@fig:kerr}{{e}{2}{}{}{}}
\@writefile{lof}{\contentsline {figure}{\numberline {1}{\ignorespaces Phase space diagrams of gate progression from (a)-(e). Taken from \cite  {hayman_hybrid_2022}.\relax }}{2}{}}
\newlabel{fig:CV_gate_progression}{{1}{2}{}{}{}}
\citation{crooks_gradients_2019}
\citation{mitarai_quantum_2018,schuld_evaluating_2019}
\@writefile{lof}{\contentsline {figure}{\numberline {2}{\ignorespaces (a) Plots showing the Fock state trace of networks as different normalization techniques are applied. (b) Demonstration of the Poisson distributions of a normalized and denormalized qumode. (c) The loss of the networks seen in (a) are plotted. Networks with good normalization or low regularization perform the best.\relax }}{3}{}}
\newlabel{fig:trace_verification}{{2}{3}{}{}{}}
\@writefile{toc}{\contentsline {section}{\numberline {III}State Trace Normalization Techniques}{3}{}}
\newlabel{sec:trace_normalization}{{III}{3}{}{}{}}
\@writefile{toc}{\contentsline {section}{\numberline {IV}Parameter Shift Rule}{3}{}}
\newlabel{sec:parameter_shift}{{IV}{3}{}{}{}}
\newlabel{eq:parameter_shift}{{1}{3}{}{}{}}
\citation{killoran_strawberry_2019}
\newlabel{eq:S}{{2}{4}{}{}{}}
\newlabel{eq:S_grad}{{3}{4}{}{}{}}
\@writefile{toc}{\contentsline {section}{\numberline {V}Hybrid Network Operation}{4}{}}
\newlabel{sec:hybrid_network_operation}{{V}{4}{}{}{}}
\@writefile{toc}{\contentsline {section}{\numberline {VI}Raw Loss Curves}{5}{}}
\@writefile{lof}{\contentsline {figure}{\numberline {3}{\ignorespaces Raw hybrid network training data.\relax }}{5}{}}
\newlabel{fig:hybrid_raw_data}{{3}{5}{}{}{}}
\citation{pedregosa_scikit-learn_2011}
\@writefile{lof}{\contentsline {figure}{\numberline {4}{\ignorespaces Raw classical network training data.\relax }}{6}{}}
\newlabel{fig:classical_raw_data}{{4}{6}{}{}{}}
\@writefile{toc}{\contentsline {section}{\numberline {VII}Encoding Comparison}{6}{}}
\newlabel{fig:encoding_comparison}{{\caption@xref {fig:encoding_comparison}{ on input line 280}}{6}{}{}{}}
\@writefile{toc}{\contentsline {section}{\numberline {VIII}PCA and Linear Fitting}{6}{}}
\newlabel{sec:linear_fitting}{{VIII}{6}{}{}{}}
\@writefile{lof}{\contentsline {figure}{\numberline {5}{\ignorespaces State vector machine classification boundaries on dimensionally reduced dataset. This model achieved 0.41 training accuracy and 0.39 testing accuracy.\relax }}{7}{}}
\newlabel{fig:svm_pca}{{5}{7}{}{}{}}
\bibdata{supplementary_informationNotes,apssamp}
\bibcite{weedbrook_gaussian_2012}{{1}{}{{Weedbrook et~al.}}{{Weedbrook, Pirandola, García-Patrón, Cerf, Ralph, Shapiro, and Lloyd}}}
\bibcite{killoran_strawberry_2019}{{2}{}{{Killoran et~al.}}{{Killoran, Izaac, Quesada, Bergholm, Amy, and Weedbrook}}}
\bibcite{kok_introduction_2010}{{3}{}{{Kok and Lovett}}{{}}}
\bibcite{gerry_introductory_2005}{{4}{}{{Gerry and Knight}}{{}}}
\bibcite{hayman_hybrid_2022}{{5}{}{{Hayman}}{{}}}
\bibcite{crooks_gradients_2019}{{6}{}{{Crooks}}{{}}}
\bibcite{mitarai_quantum_2018}{{7}{}{{Mitarai et~al.}}{{Mitarai, Negoro, Kitagawa, and Fujii}}}
\bibcite{schuld_evaluating_2019}{{8}{}{{Schuld et~al.}}{{Schuld, Bergholm, Gogolin, Izaac, and Killoran}}}
\bibcite{pedregosa_scikit-learn_2011}{{9}{}{{Pedregosa et~al.}}{{Pedregosa, Varoquaux, Gramfort, Michel, Thirion, Grisel, Blondel, Prettenhofer, Weiss, Dubourg, Vanderplas, Passos, Cournapeau, Brucher, Perrot, and Duchesnay}}}
\bibstyle{unsrtnat}
\@writefile{lof}{\contentsline {figure}{\numberline {6}{\ignorespaces Kmeans clustering on dimensionally reduced dataset. This model achieved 0.42 training accuracy and 0.36 testing accuracy.\relax }}{8}{}}
\newlabel{fig:pca_kmeans}{{6}{8}{}{}{}}
\@writefile{toc}{\contentsline {section}{\numberline {}References}{8}{}}
\newlabel{LastBibItem}{{9}{8}{}{}{}}
\newlabel{LastPage}{{}{8}{}{}{}}
\gdef \@abspage@last{8}

\end{filecontents}
